# Supplementary material for: Palpatine: Mining Frequent Sequences for Data Prefetching in NoSQL Distributed Key-Value Stores
Source: arXiv:2002.00215 source file (2020-04-22)
Supplement: Supplementary file 1 [file appendix.tex]

\graphicspath{{appendix/}}

To support our choice of the VMSP data mining algorithm, we compare it here against other common and well-known algorithms.

\spara{Algorithms.} The sequential pattern mining algorithms that we consider for comparison are listed as follows.

%\begin{tabular}{ l c r }
%  Apriori & Pattern-growth
%  BFS & 2 & 3 \\
%  DFS & 5 & 6 \\
%  7 & 8 & 9 \\
%\end{tabular}

\begin{itemize}
	\item Apriori
	\begin{itemize}
		\item BFS: GSP
		\item DFS: Spade, Spam
	\end{itemize}
	\item Pattern-growth
	\begin{itemize}
		\item DFS: PrefixSpan
	\end{itemize}
	\item Closed Sequential Patterns: ClaSP
	\item Maximal Sequential Patterns: MaxSP, VMSP
	\item Generator Sequential Patters: VGEN
\end{itemize}

\spara{Comparison.} Figure~\ref{fig:app-time-memory} shows the time and memory used for the considered algorithms for different minimum support values. We can see that VMSP is very competitive in terms of time and memory used. PrefixSpan, which explores all sequential patterns, exhibits similar time and memory usage. However, PrefixSpan generates roughly two orders of magnitude more sequences that VMSP, as depicted in Figure~\ref{fig:app-sequences}. This means that \name would have to store a larger amount of metadata, in the Pattern Metastore component (cf. Section~\ref{sect:architecture}), than it would with VMSP. MaxSP generates the fewer sequences, but it is not efficient in terms of memory usage.

\begin{figure*}
	\centering
	\begin{subfigure}[t]{0.49\textwidth}
		\centering
	  \includegraphics[width=0.8\columnwidth]{time}
	  \caption{Time}
	\end{subfigure}
	\begin{subfigure}[t]{0.49\textwidth}
			\centering
	  \includegraphics[width=0.8\columnwidth]{memory}
	  \caption{Memory}
	\end{subfigure}
	\caption{Time and memory}
	\label{fig:app-time-memory}
\end{figure*}

\begin{figure}
	\centering
	\includegraphics[width=0.8\columnwidth]{sequences}
	\caption{Number of sequences}
	\label{fig:app-sequences}
\end{figure}

In order to compare the gains of \name using different data mining algorithms, we compare now VMSP, that only generates maximal patterns, against an algorithm that generates all patterns - as a concrete instance we resorted to PrefixSpan since it is one of the algorithms that generated the largest number of sequences while exhibiting similar performance (time, memory) with respect to VMSP. For this particular comparison we used a minimum support of 0.01 (i.e., 1\%).

We can see that PrefixSpan is on a par with VMSP in terms of precision (Figure~\ref{fig:app-precision}), hit-rate (Figure~\ref{fig:app-hit-rate}), latency (Figure~\ref{fig:app-latency}), throughput (Figure~\ref{fig:app-throughput}), and runtime (Figure~\ref{fig:app-runtime}). This comes with no surprise, since maximal sequences generated by VMSP should be contained in all sequences generated by PrefixSpan. However, \name has to account with a higher number of trees and sequences, that are mostly useless for the problem at hand, in Pattern Metastore with PrefixSpan. This would make applications, that make use of \name, to occupy two orders of magnitude more memory than with VMSP, which is a significant waste given that most of the sequences in PrefixSpan (subsequences of other larger sequences) are useless for the prefetching as explained before in Section~\ref{sect:data-mining}.

\begin{figure}
	\centering
	\begin{subfigure}[t]{0.49\columnwidth}
	  \includegraphics[width=\columnwidth]{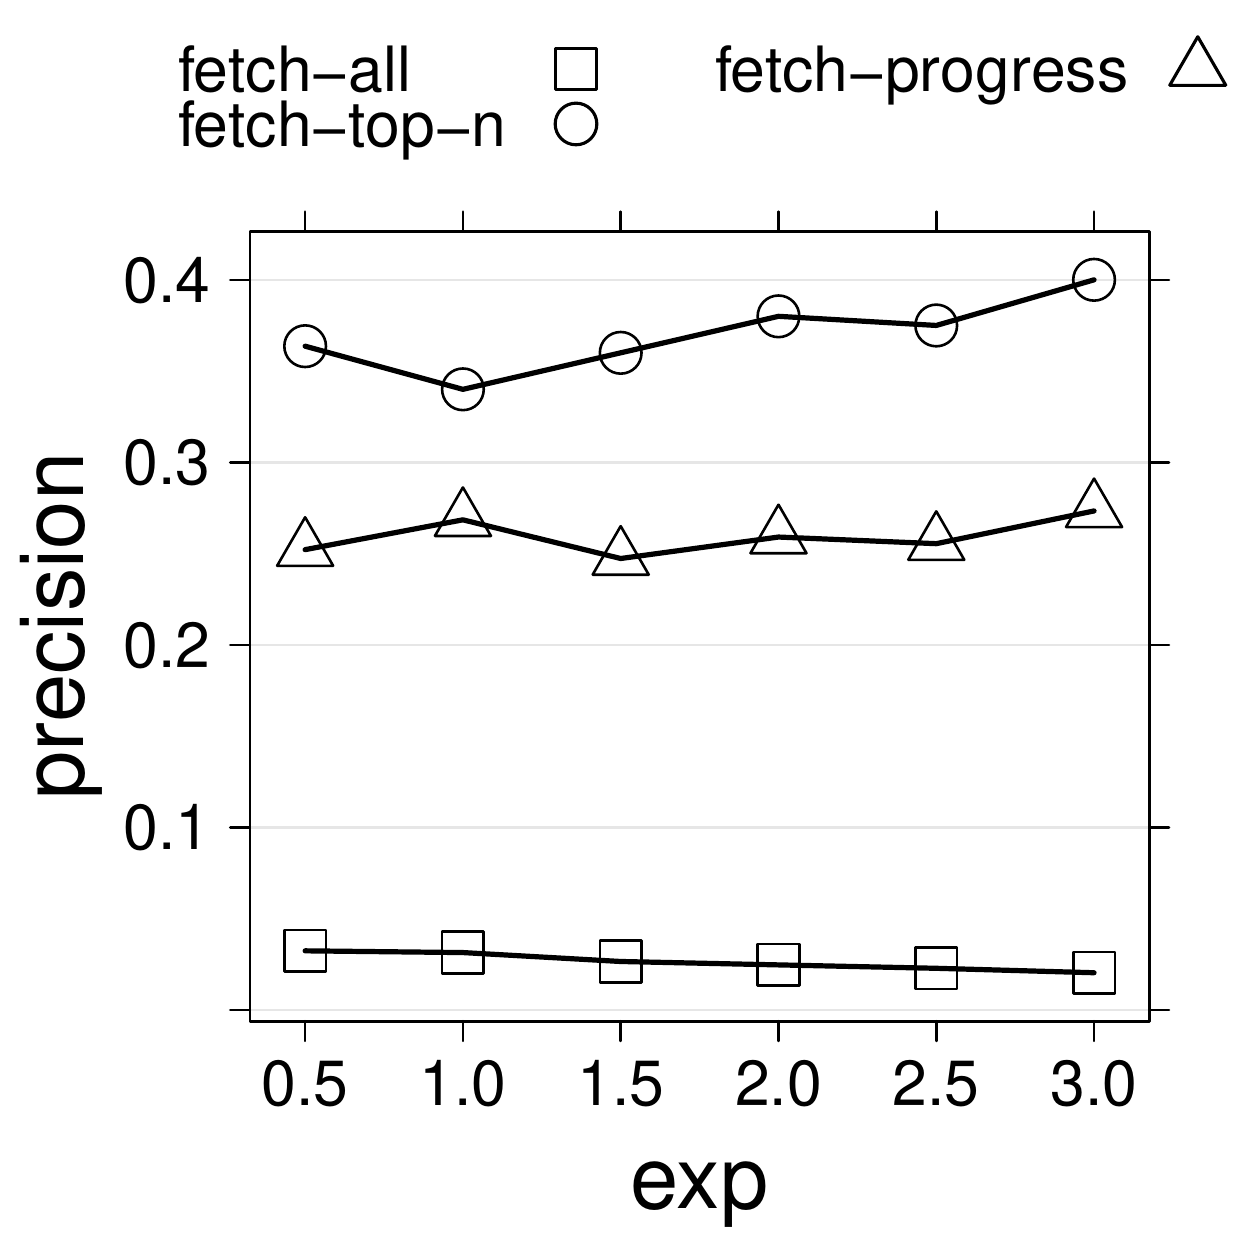}
	  \caption{PrefixSpan}
	  \label{fig:precision}
	\end{subfigure}
	\begin{subfigure}[t]{0.49\columnwidth}
	  \includegraphics[width=\columnwidth]{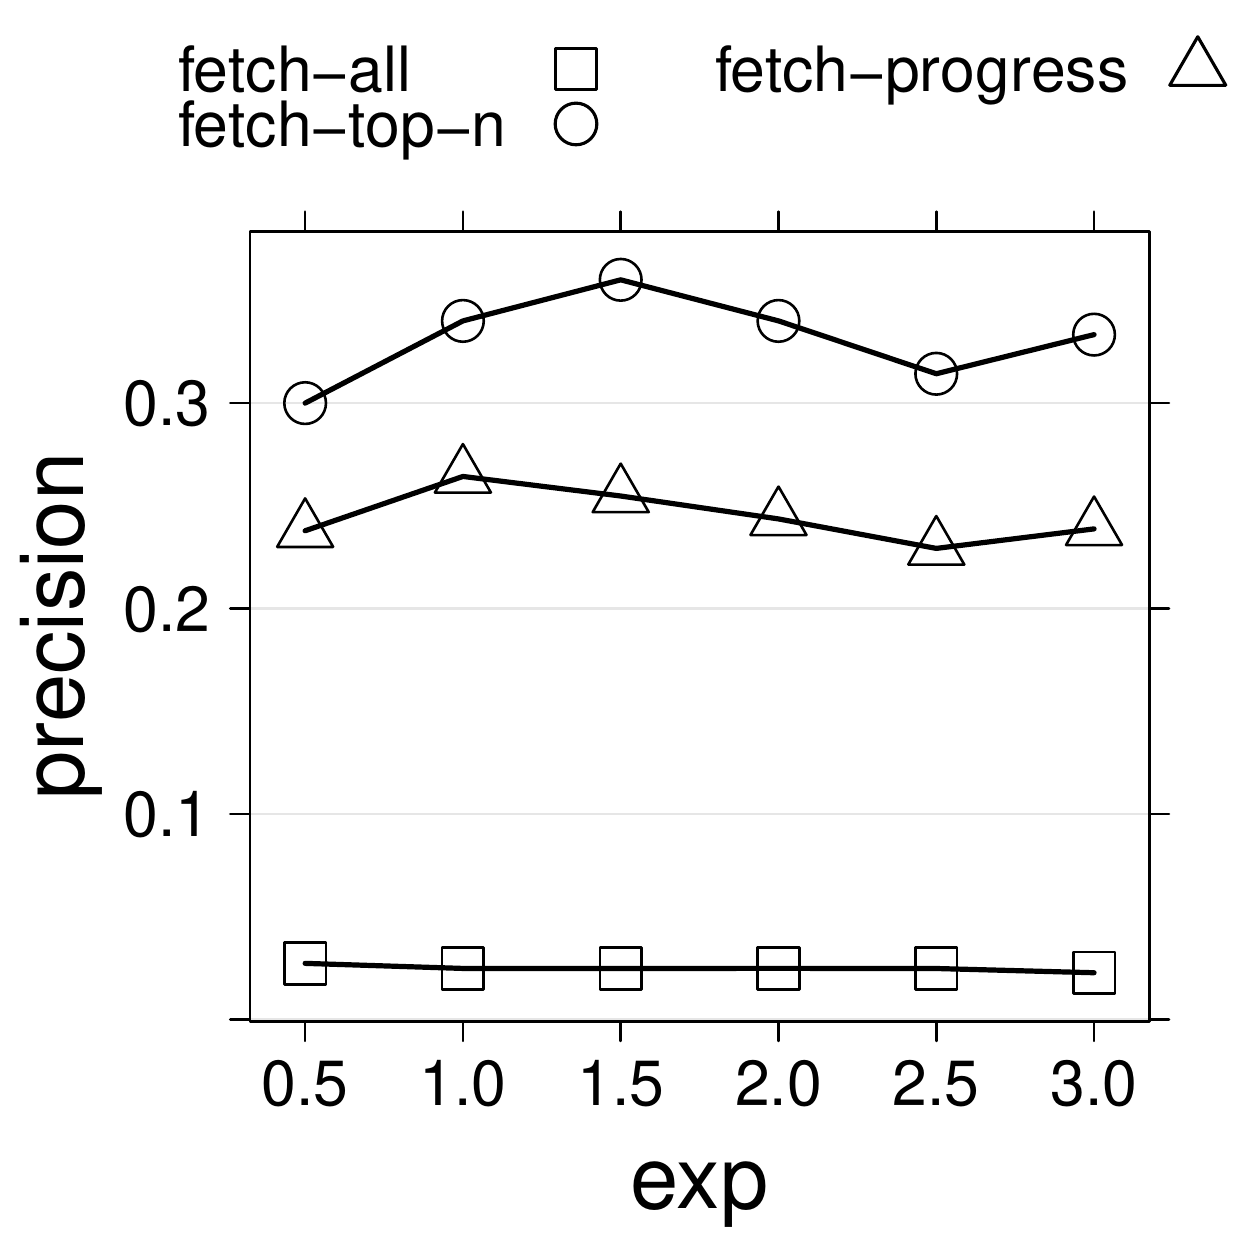}
	  \caption{VMSP}
	  \label{fig:precision}
  	\end{subfigure}
	\caption{Prefetch precision}
	\label{fig:app-precision}
\end{figure}

\begin{figure}
	\centering
	\begin{subfigure}[t]{0.49\columnwidth}
  	  \includegraphics[width=\columnwidth]{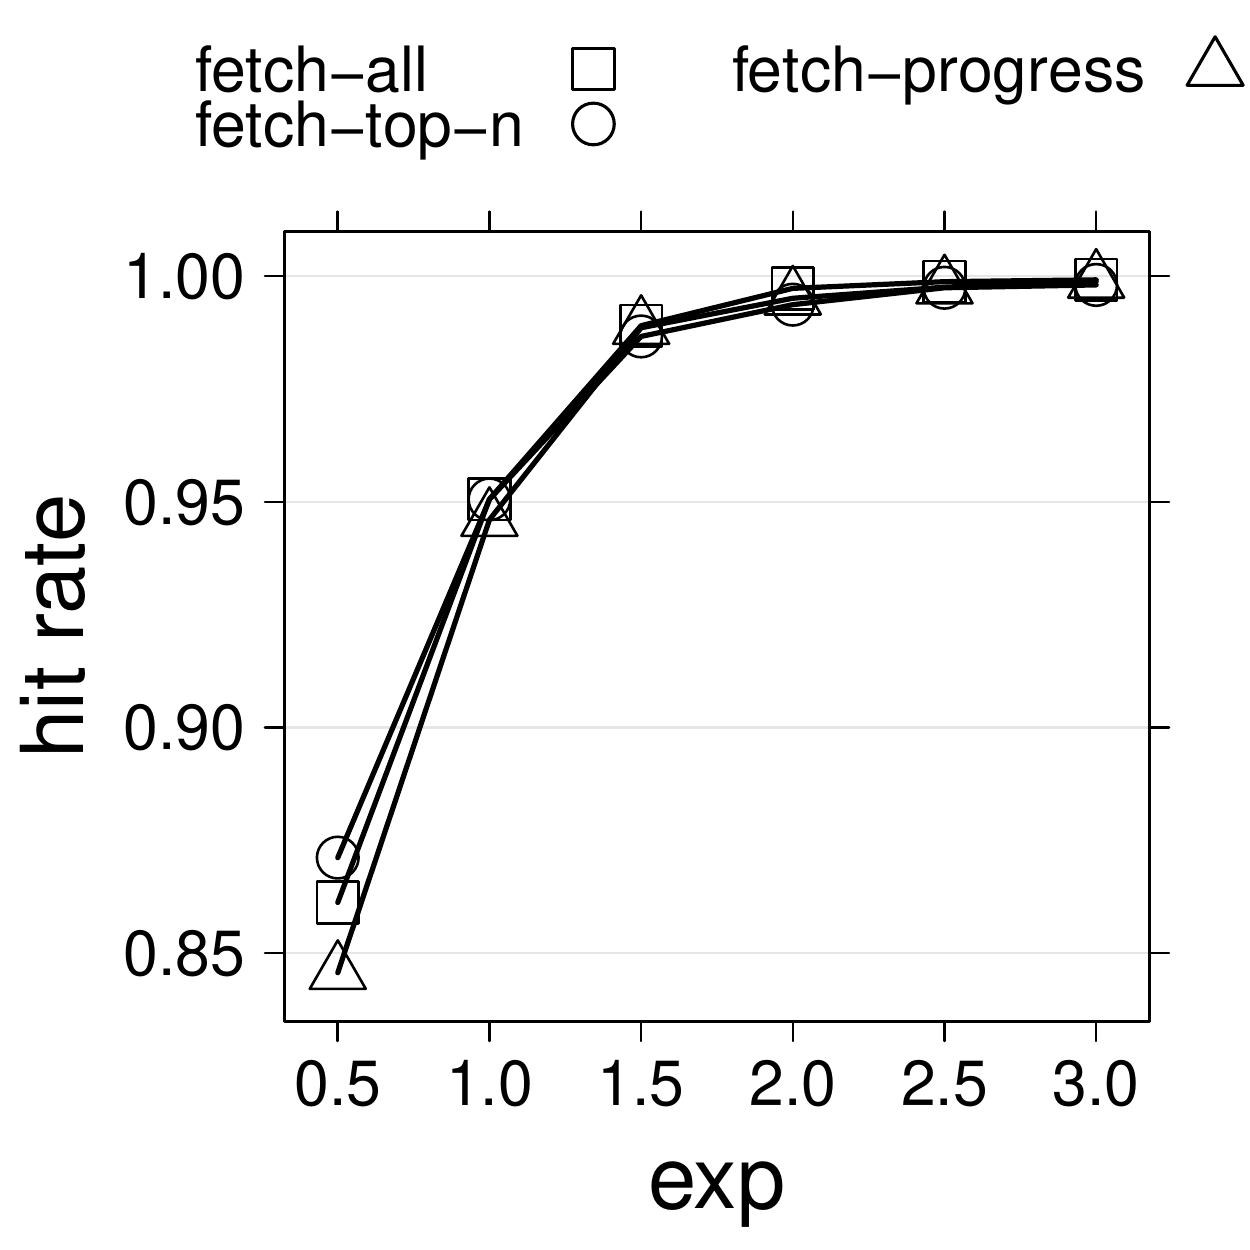}
  	  \caption{PrefixSpan}
  	  \label{fig:hit-rate}
	\end{subfigure}
	\begin{subfigure}[t]{0.49\columnwidth}
  	  \includegraphics[width=\columnwidth]{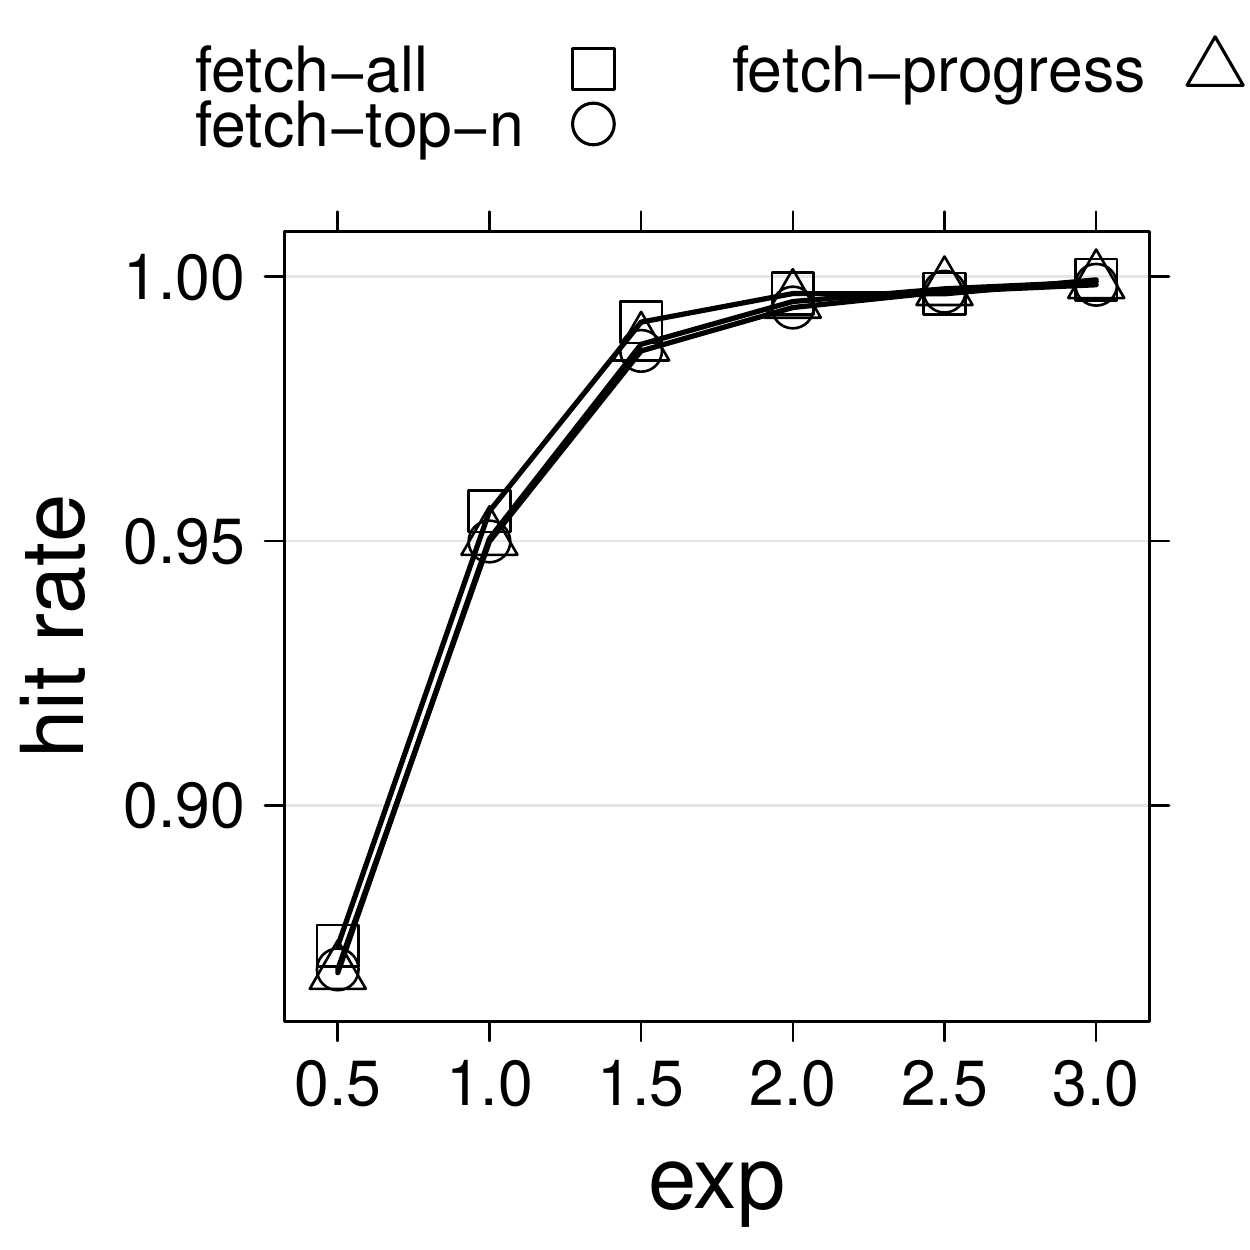}
  	  \caption{VMSP}
  	  \label{fig:hit-rate}
  	\end{subfigure}
	\caption{cache hit rate}
	\label{fig:app-hit-rate}
\end{figure}

\begin{figure*}
	\centering
	\begin{subfigure}[t]{0.25\textwidth}
	  \includegraphics[width=\textwidth]{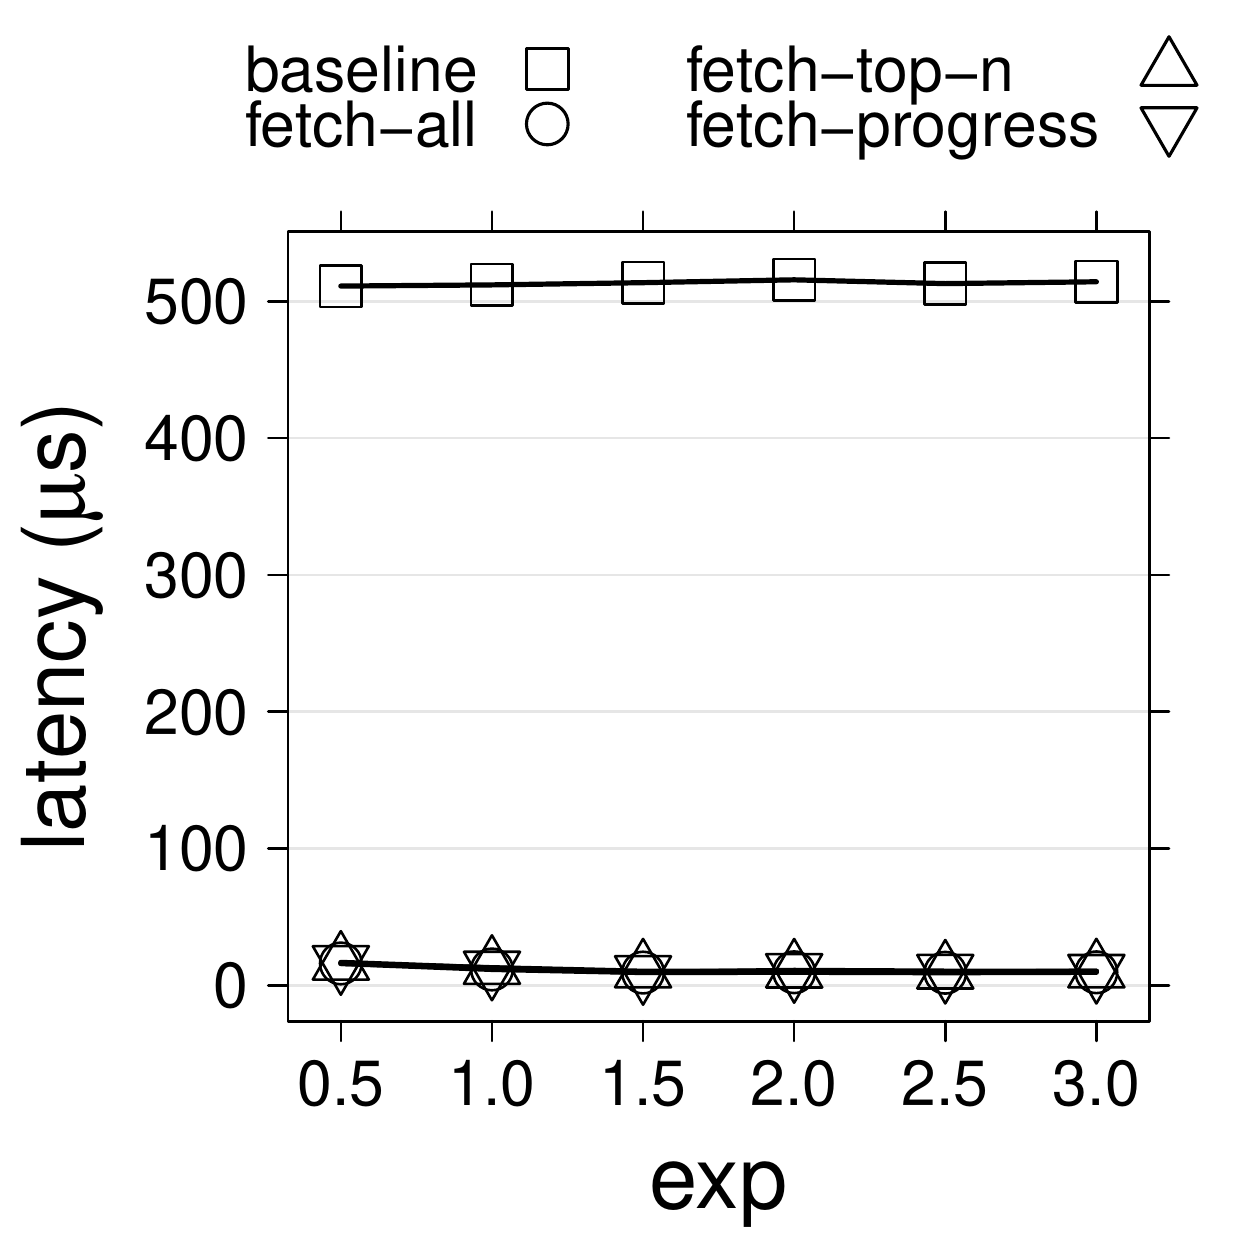}
	  \caption{PrefixSpan Median}
	  \label{fig:latency-50}
	\end{subfigure}
	\begin{subfigure}[t]{0.25\textwidth}
      \includegraphics[width=\textwidth]{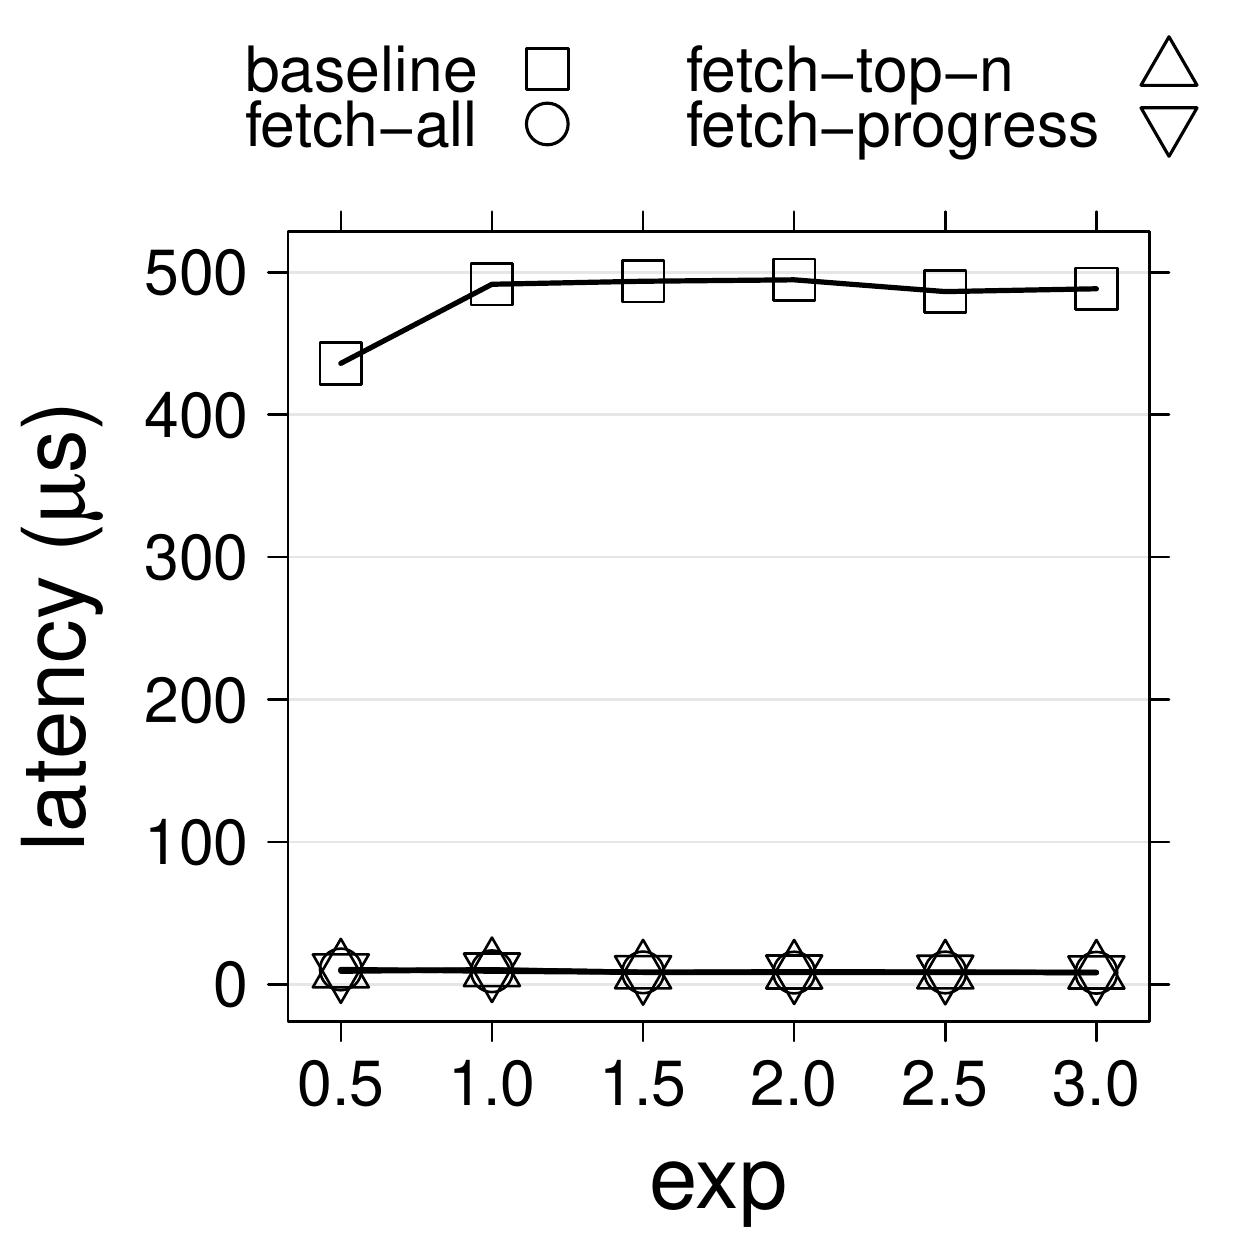}
      \caption{PrefixSpan 5th percentile}
      \label{fig:latency-5}
	\end{subfigure}	  
	\begin{subfigure}[t]{0.25\textwidth}
      \includegraphics[width=\textwidth]{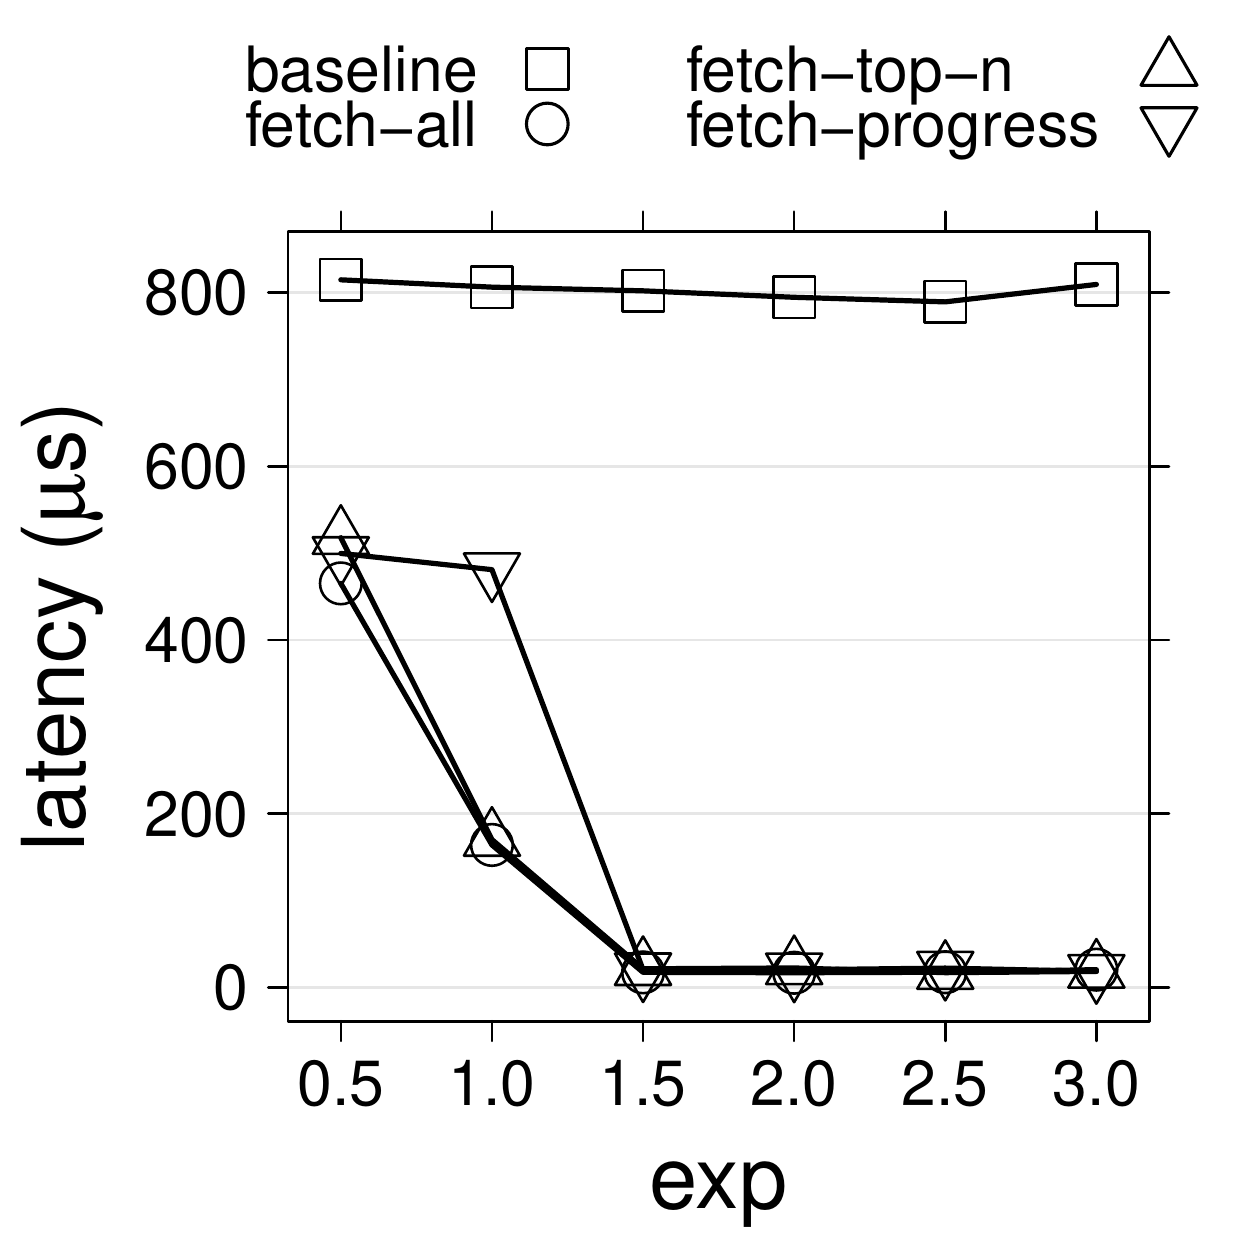}
      \caption{PrefixSpan 95th percentile}
      \label{fig:latency-95}
	\end{subfigure}
		\begin{subfigure}[t]{0.25\textwidth}
	  \includegraphics[width=\textwidth]{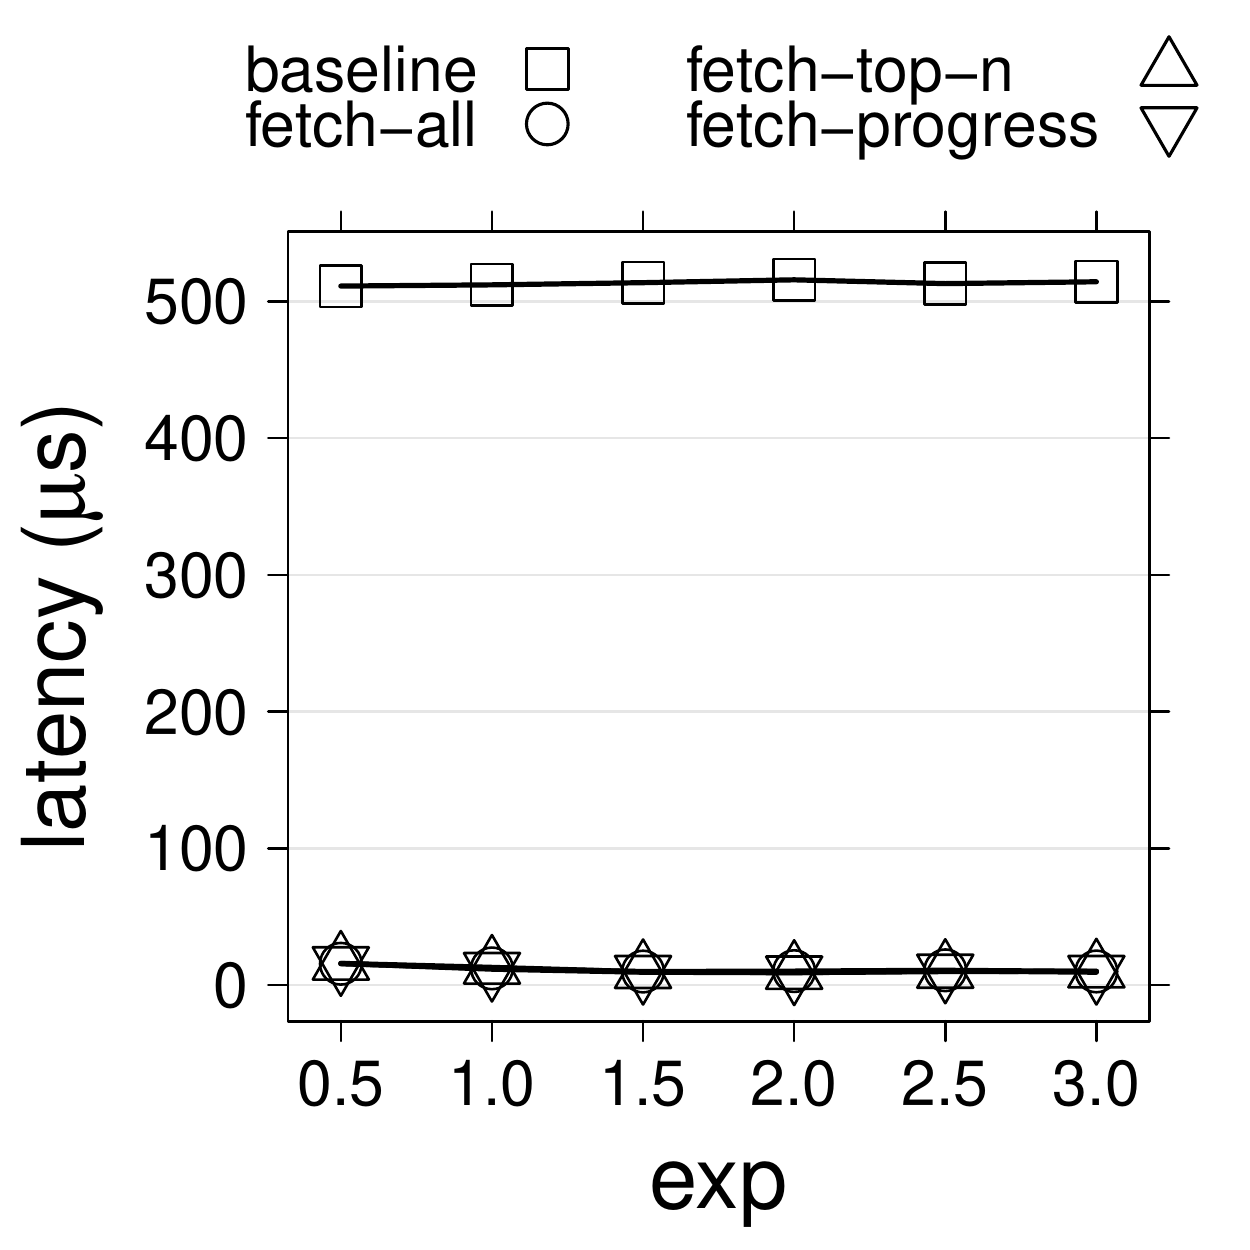}
	  \caption{VMSP Median}
	  \label{fig:latency-50}
	\end{subfigure}
	\begin{subfigure}[t]{0.25\textwidth}
      \includegraphics[width=\textwidth]{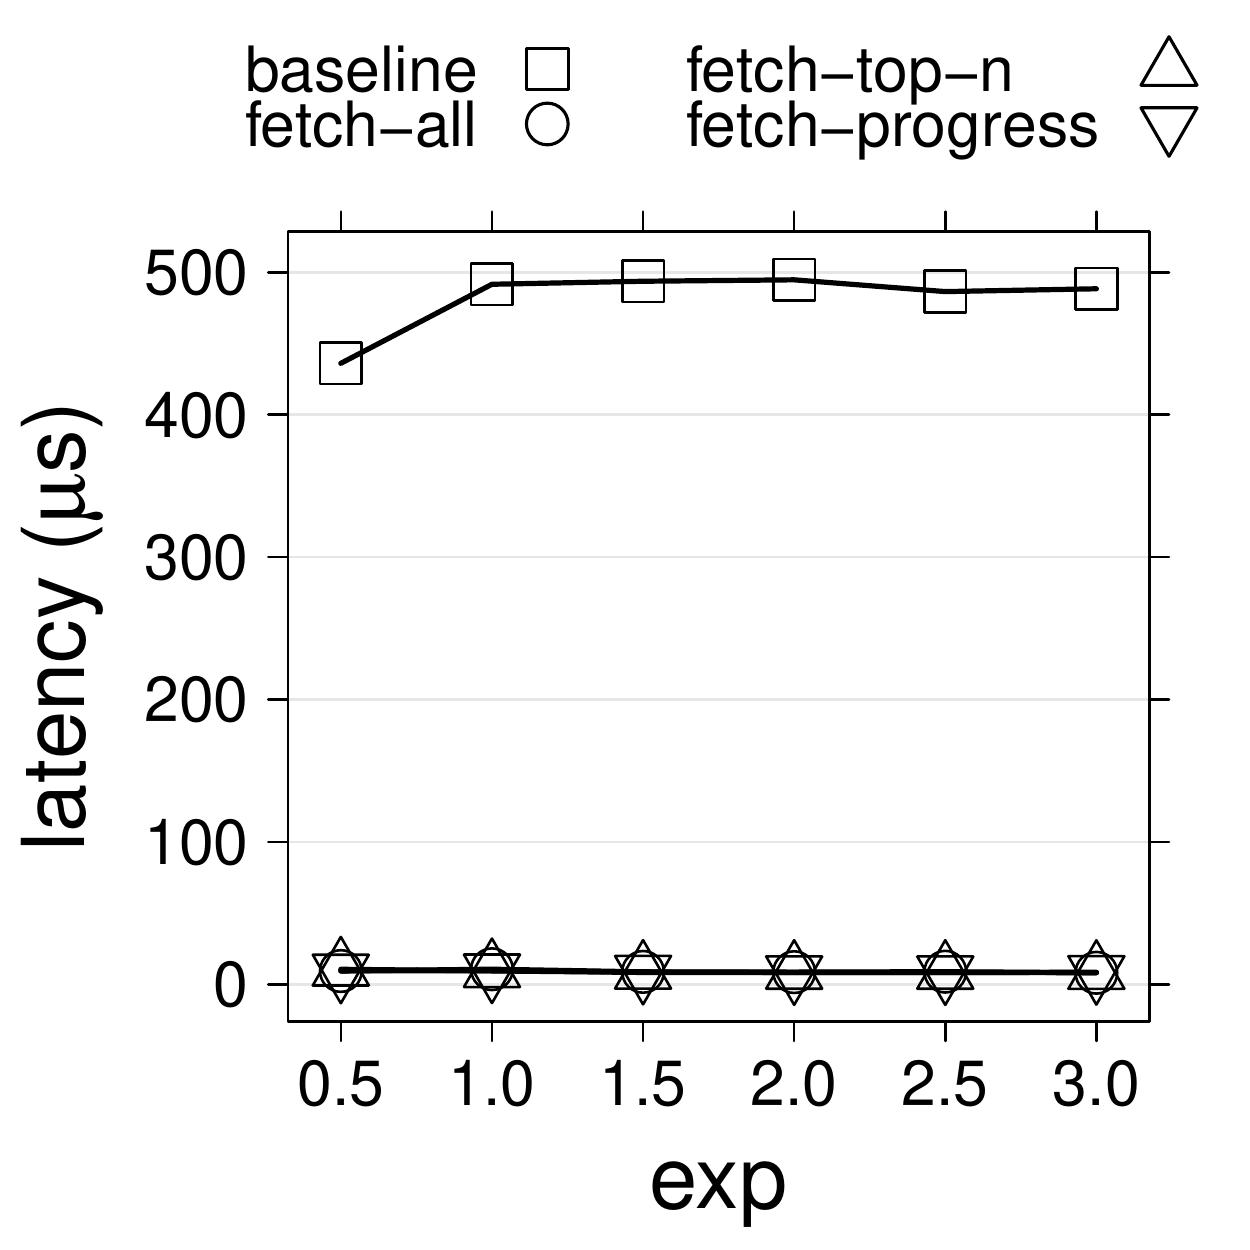}
      \caption{VMSP 5th percentile}
      \label{fig:latency-5}
	\end{subfigure}	  
	\begin{subfigure}[t]{0.25\textwidth}
      \includegraphics[width=\textwidth]{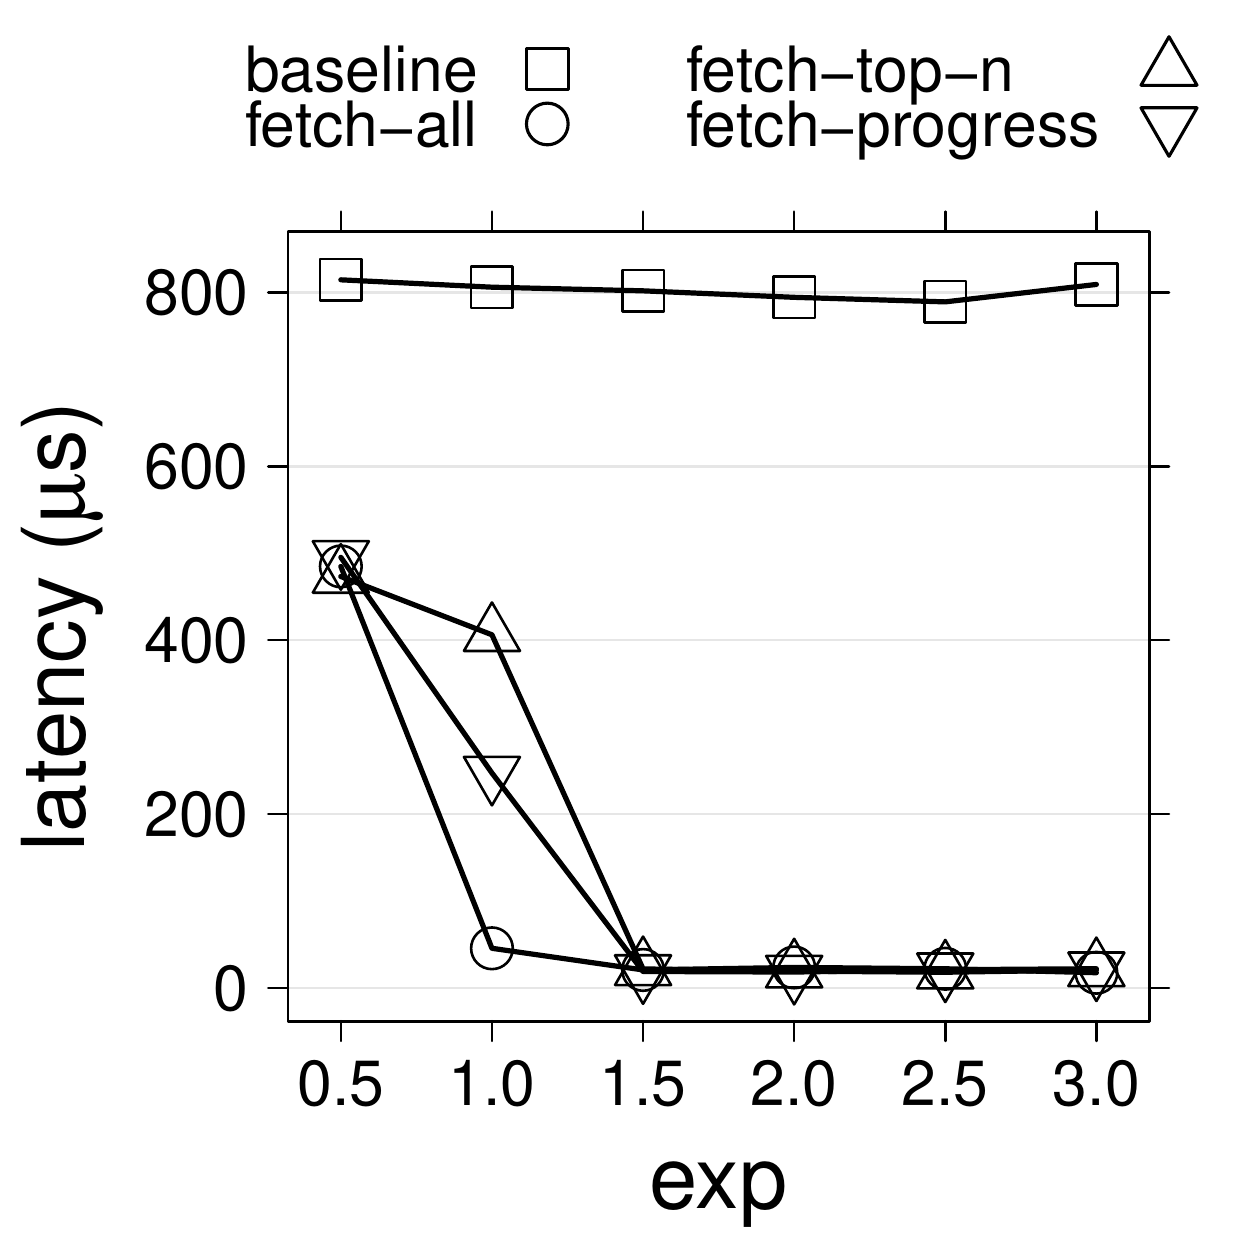}
      \caption{VMSP 95th percentile}
      \label{fig:latency-95}
	\end{subfigure}	  
	\caption{Operation latency}
	\label{fig:app-latency}
\end{figure*}

\begin{figure*}
	\centering
	\begin{subfigure}[t]{0.25\textwidth}
	  \includegraphics[width=\textwidth]{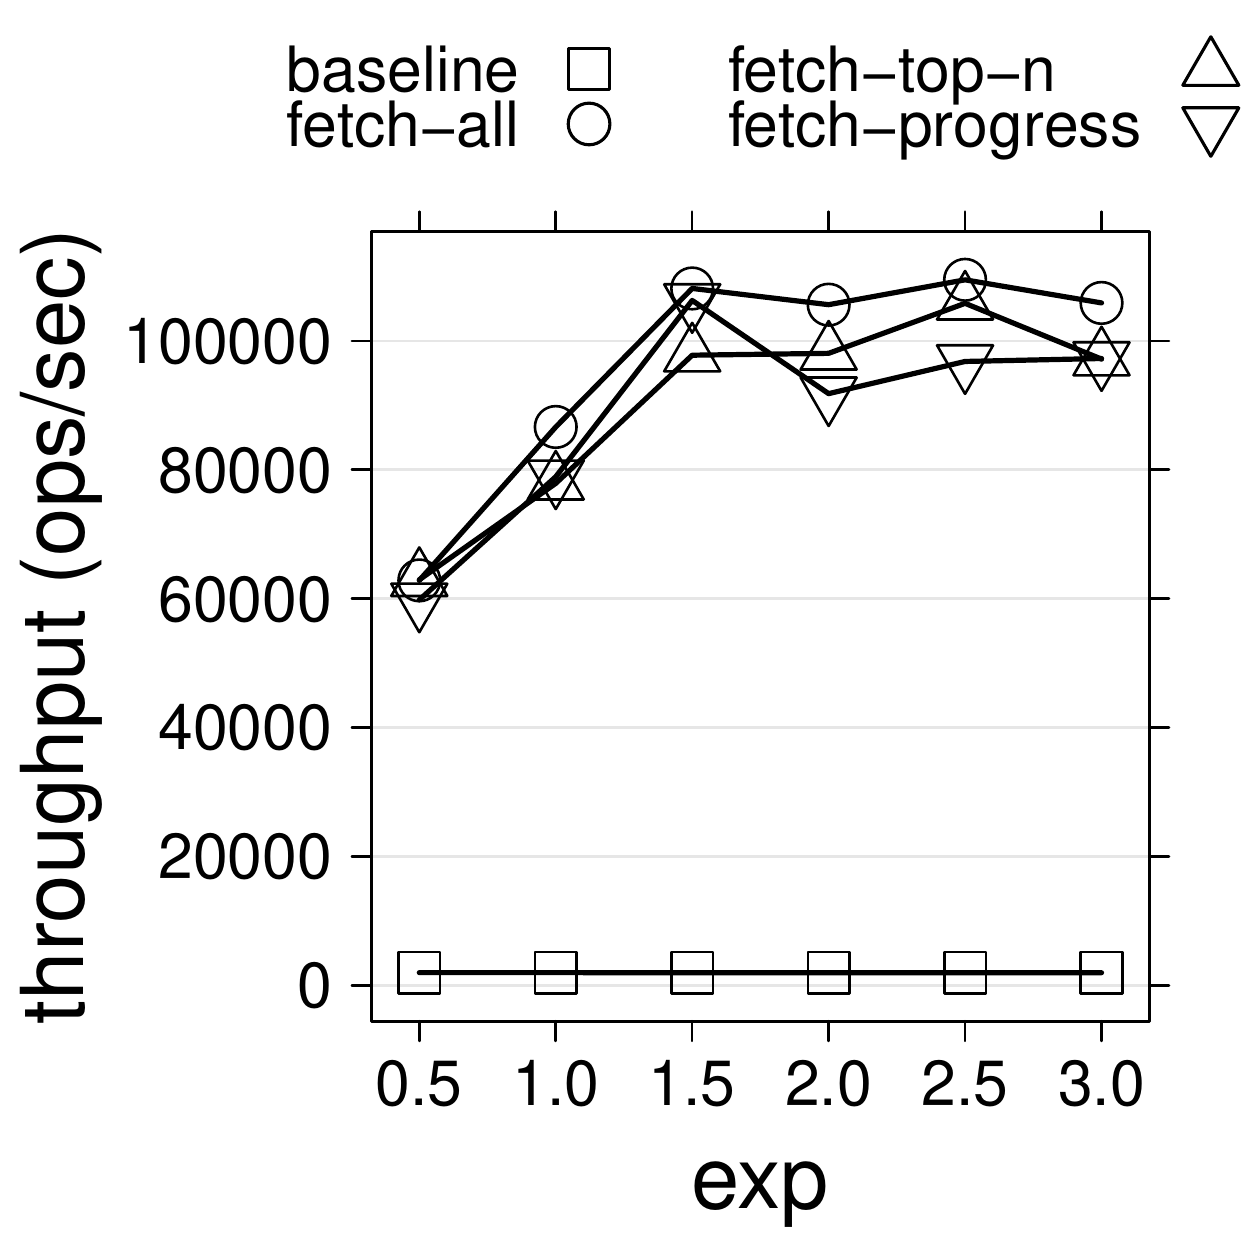}
	  \caption{PrefixSpan Median}
	  \label{fig:throughput-50}
	\end{subfigure}
	\begin{subfigure}[t]{0.25\textwidth}
      \includegraphics[width=\textwidth]{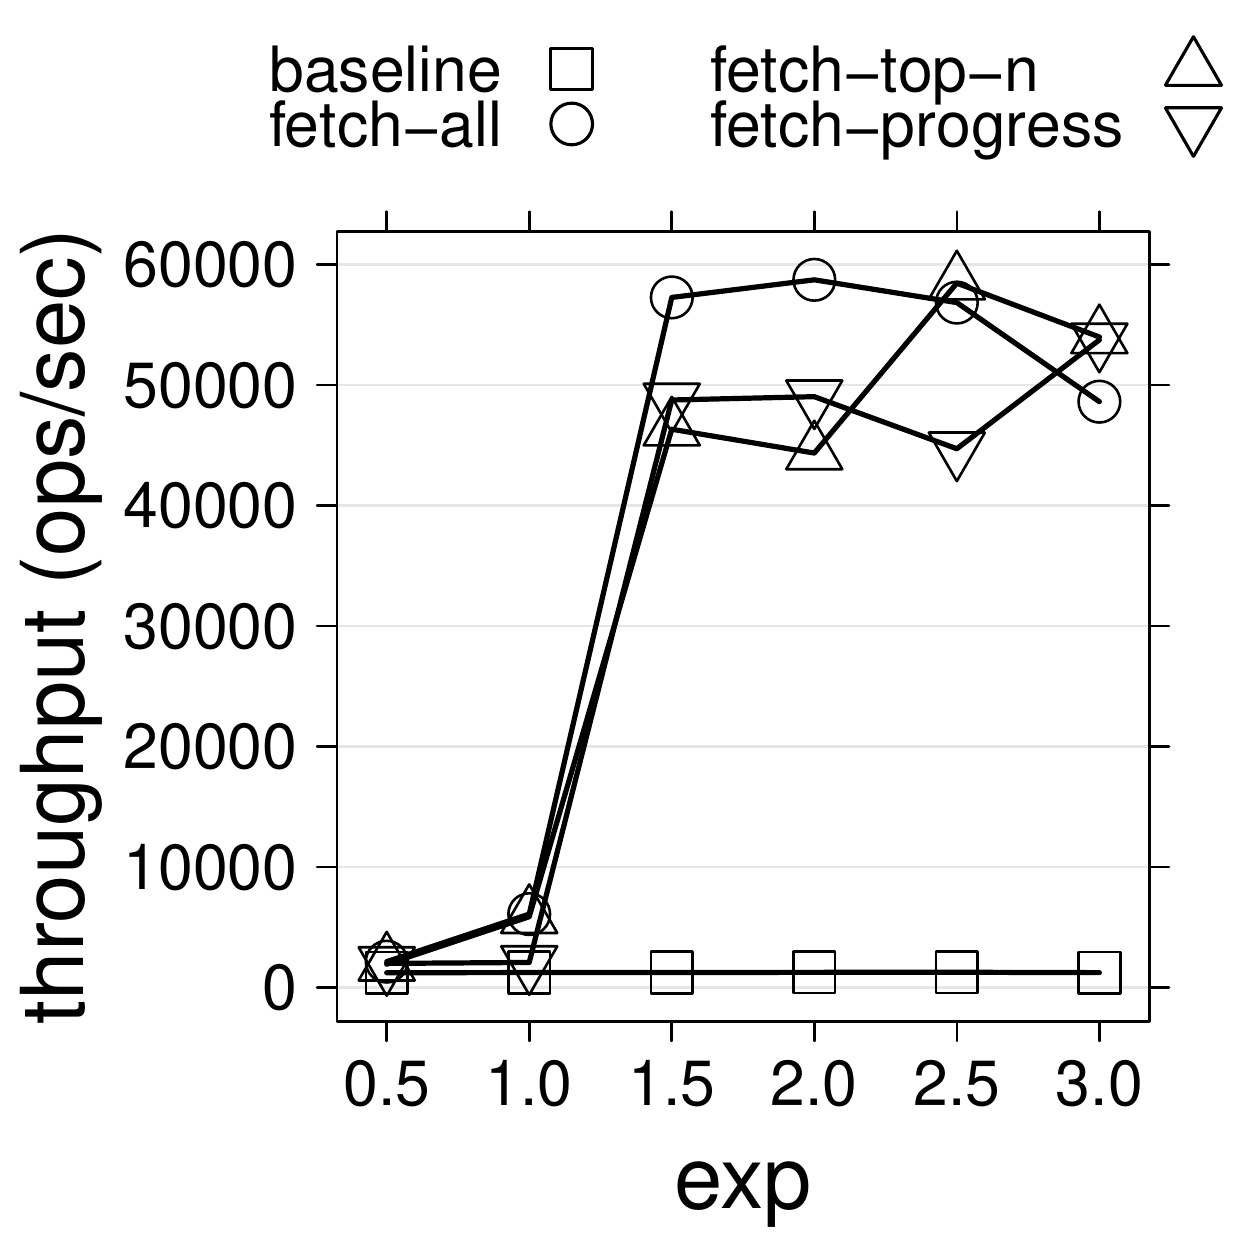}
      \caption{PrefixSpan 5th percentile}
      \label{fig:throughput-5}
	\end{subfigure}	  
	\begin{subfigure}[t]{0.25\textwidth}
      \includegraphics[width=\textwidth]{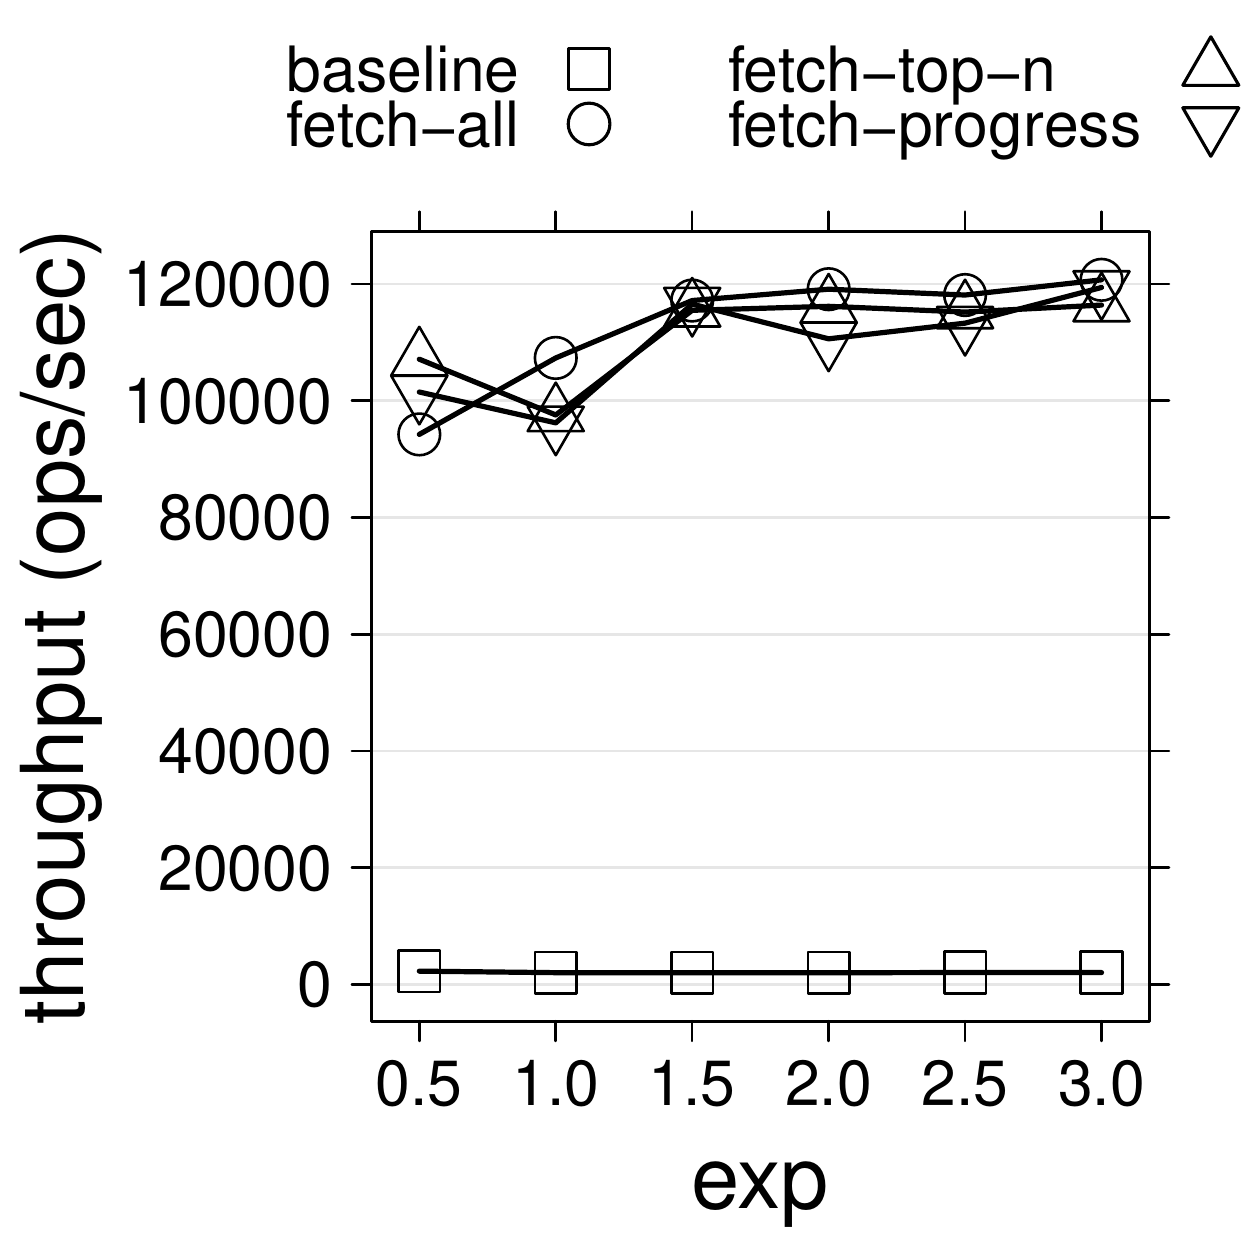}
      \caption{PrefixSpan 95th percentile}
      \label{fig:throughput-95}
	\end{subfigure}	  
	\begin{subfigure}[t]{0.25\textwidth}
	  \includegraphics[width=\textwidth]{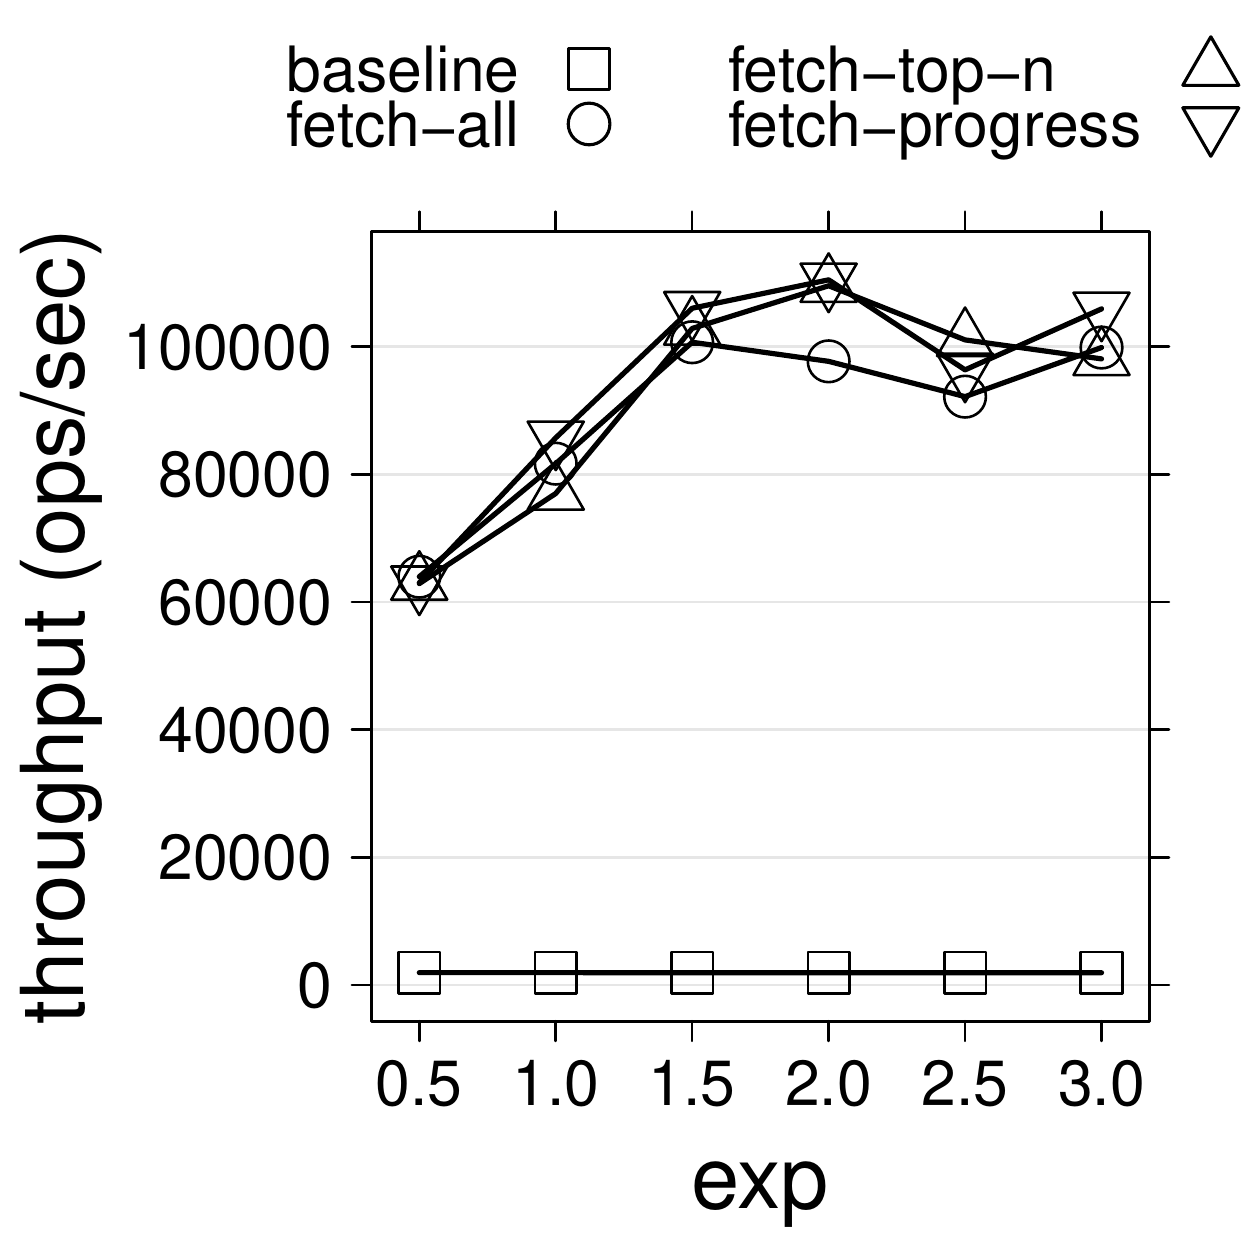}
	  \caption{VMSP Median}
	  \label{fig:throughput-50}
	\end{subfigure}
	\begin{subfigure}[t]{0.25\textwidth}
      \includegraphics[width=\textwidth]{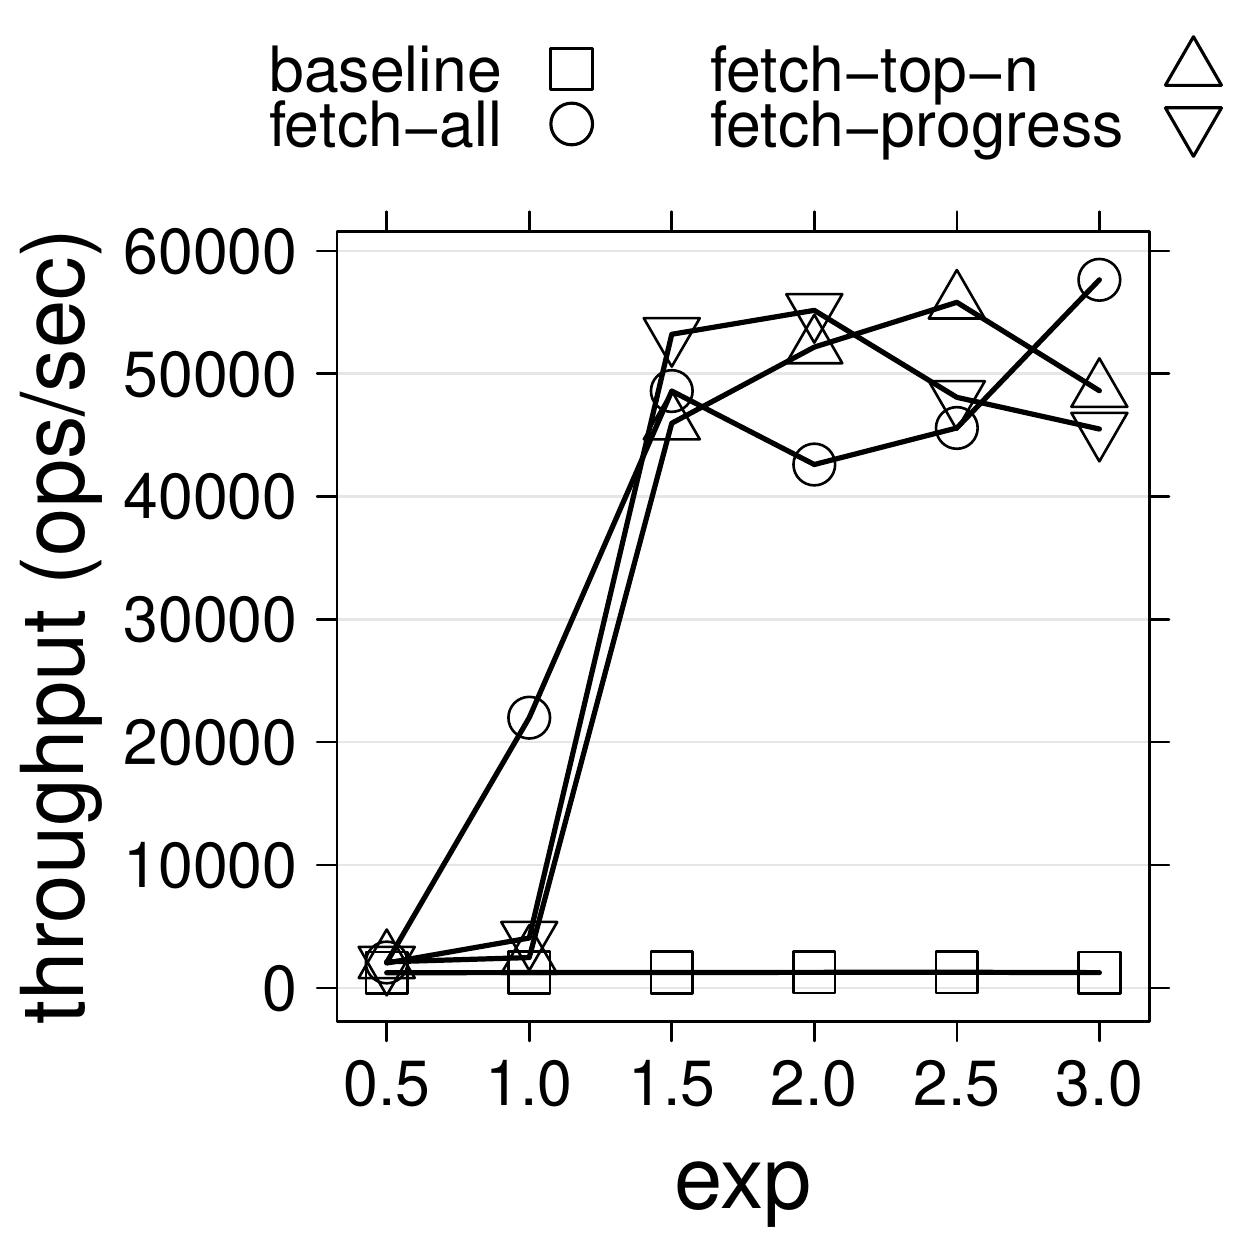}
      \caption{VMSP 5th percentile}
      \label{fig:throughput-5}
	\end{subfigure}	  
	\begin{subfigure}[t]{0.25\textwidth}
      \includegraphics[width=\textwidth]{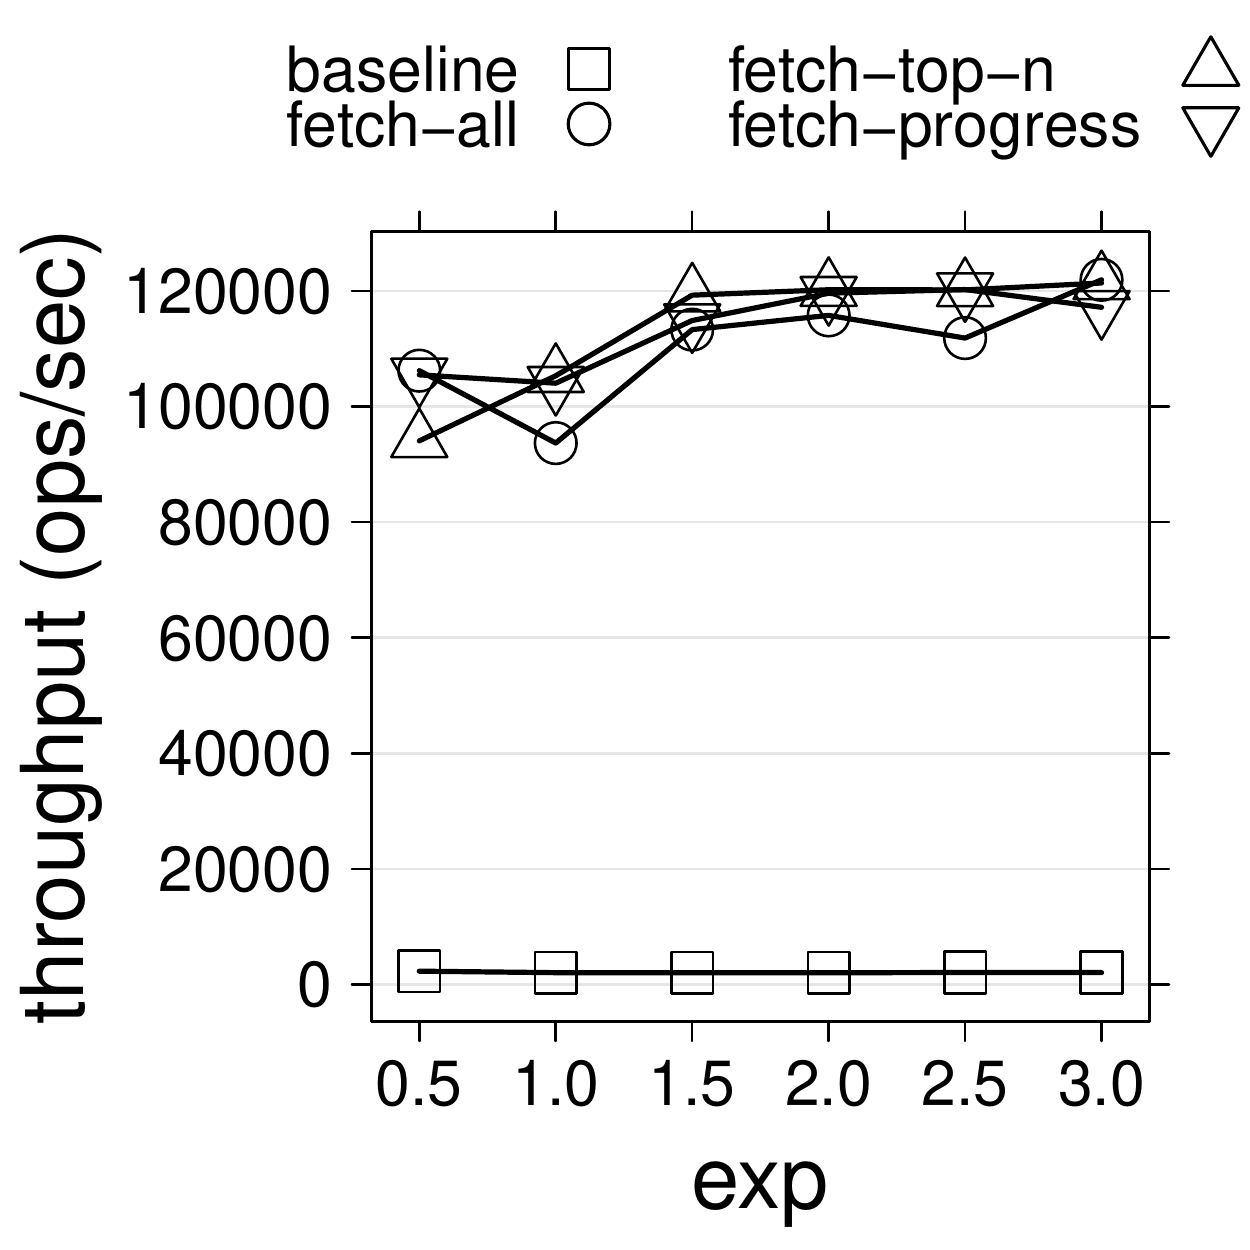}
      \caption{VMSP 95th percentile}
      \label{fig:throughput-95}
	\end{subfigure}	  	
	
	\caption{Operation throughput}
	\label{fig:app-throughput}
\end{figure*}

\begin{figure*}
	\centering
	\begin{subfigure}[t]{0.49\textwidth}
	\centering
		\includegraphics[width=0.8\columnwidth]{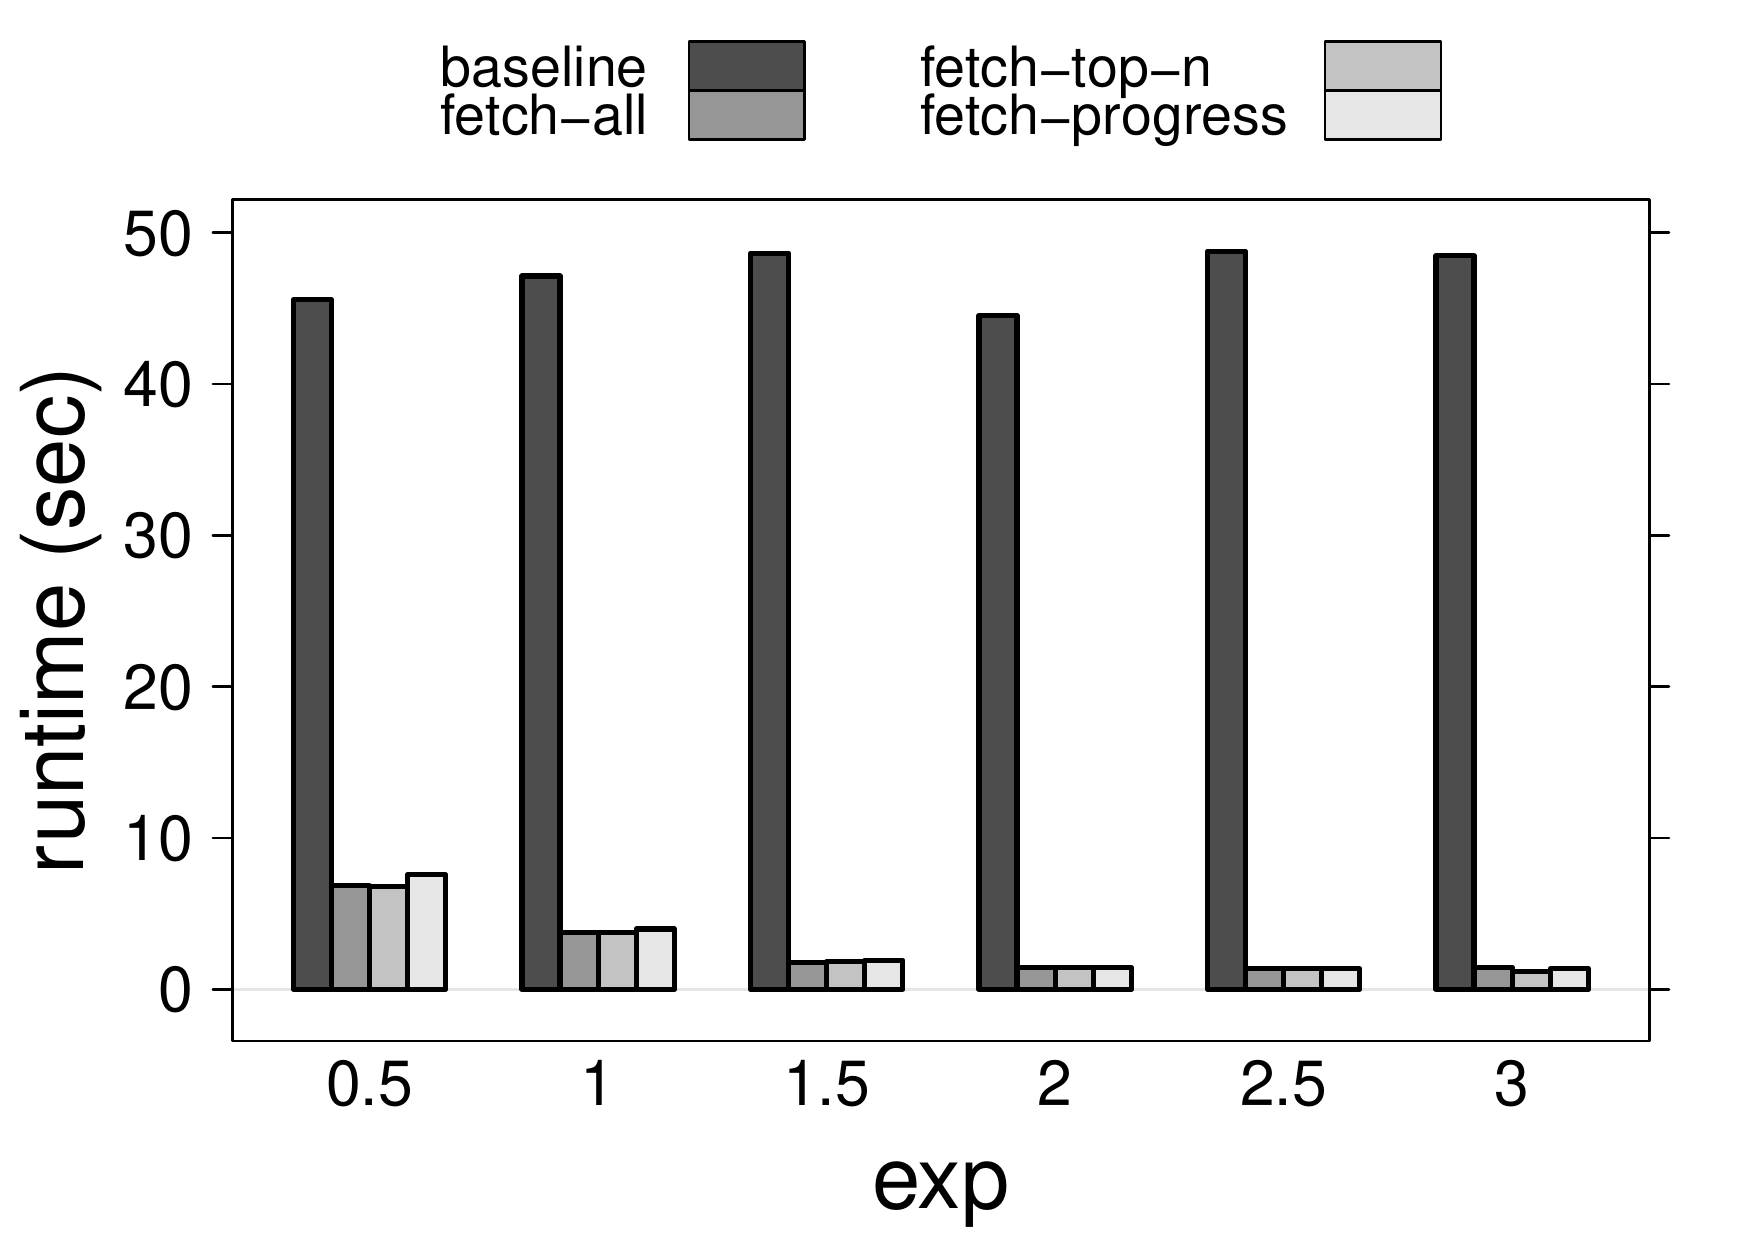}
		\caption{PrefixSpan}
	\end{subfigure}
	\begin{subfigure}[t]{0.49\textwidth}
	\centering
		\includegraphics[width=0.8\columnwidth]{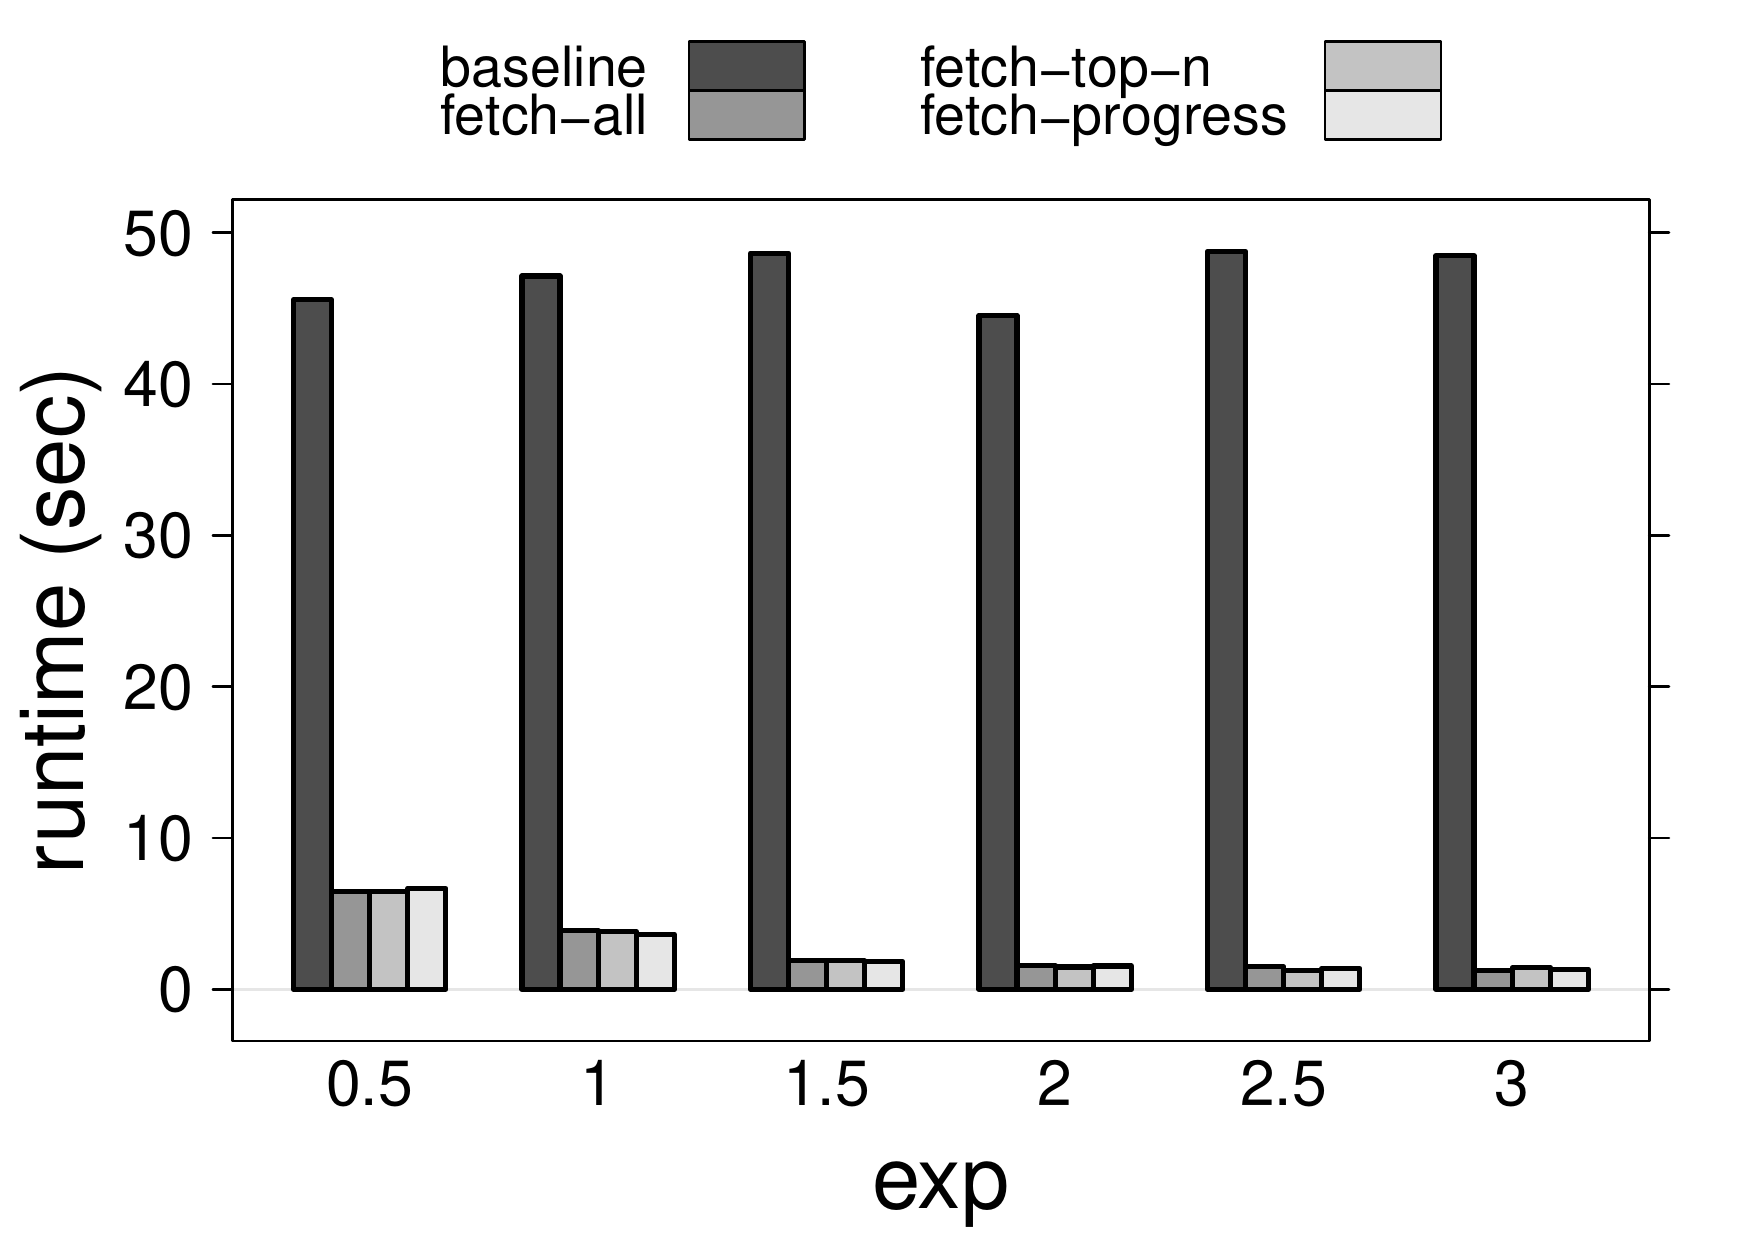}
		\caption{VMSP}
	\end{subfigure}
	\caption{Runtime}
	\label{fig:app-runtime}
\end{figure*}
